# Supplementary material for: Critical photoinduced reflectivity relaxation dynamics in single-layer Bi-based cuprates near the pseudogap end point
Source: arXiv:2508.21298 ancillary file (2026-09-03)
Supplement: Supplementary file 1 [file Suppl-ODPG.pdf]

# Supplemental Material for:
# Critical photoinduced reflectivity relaxation dynamics in single-layer Bi-based cuprates near the pseudogap end point

T. Shimizu,[1] R. Tobise,[1] T. Kurosawa,[1] S. Tsuchiya,[1] M. Oda,[2]
Y. Toda,[1] V. V. Kabanov,[3] D. Mihailovic,[3] and T. Mertelj[3]

[1] *Department of Applied Physics, Hokkaido University, Sapporo 060-8628, Japan.*
[2] *Department of Physics, Hokkaido University, Sapporo 060-0810, Japan.*
[3] *Complex Matter Dept., Jozef Stefan Institute, Jamova 39, Ljubljana, SI-1000, Slovenia.*
(Dated: August 25, 2025)

## I. MAGNETIC SUSCEPTIBILITY OF THE SAMPLES

The results of magnetic susceptibility measurements for OPD34 and three Pb-substituted Bi2201 samples (VOD10 with $T_c = 10$ K, VOD7 with $T_c = 7$ K, and the non-superconducting VOD0) are presented in Figs. S1(a) and (b). In Fig. S1(b), the mass susceptibility is shown for comparison. For clarity, the data for VOD7 have been scaled by a factor of $10^{-1}$. The mass susceptibility of VOD7 is approximately $-1.5 \times 10^{-1}$ emu/g at $T = 3.5$ K, indicating an estimated superconducting volume fraction close to 100%. The mass susceptibility of VOD10 at $T = 5$ K is approximately $-1.0 \times 10^{-2}$ emu/g, corresponding to a superconducting volume fraction of $\sim 10\%$. As shown in Fig. S1(c), the doping levels of these three samples correspond to the pre-PGED, the beyond-PGED, and the beyond-SC endpoint doping, respectively.

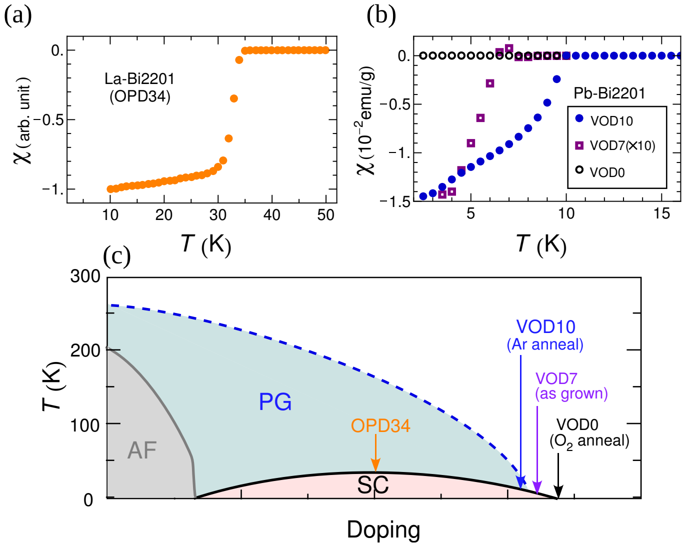


FIG. S1. (a) Temperature dependence of magnetic susceptibility of optimally-doped La-Bi2201 (OPD34) and (b) overdoped Pb-Bi2201 samples. (c) Temperature-doping phase diagram of Bi2201. Superconducting phase transition temperatures $T_c^m$ is estimated to be 34 K for OPD34K, 10 K for the sample annealed in Ar atmosphere (VOD10), and 7 K for the as-grown sample (VOD7), respectively, while the sample annealed in $O_2$ atmosphere (VOD0) shows no superconducting transition down to $T = 2.5$ K. A possible onset temperature of the pseudogap is indicated by the dashed line [1].

## II. PHOTOEXCITATION FLUENCE DEPENDENCE

Figure S2 shows the transient reflectivity $\Delta R/R$ at selected fluences for each sample. For reference, the $\Delta R/R$ at the lowest fluence is displayed in the bottom of each panel. The transient data for OPD34 [Fig. S2(a)] were measured at $T = 50$ K, where superconductivity is fully suppressed and the pseudogap state is dominant, whereas the data for VOD samples [Figs. S2 (b)–(d)] were obtained at temperatures near $T_c$. The negative transient reflectivity signal (pseudogap response) dominates in OPD34 (Fig. S2(a)) and VOD10 (Fig. S2(b)), whereas only a positive transient

signal is observed in VOD7 (Fig. S2(c)) and VOD0 (Fig. S2(d)). The oscillatory components, which become prominent at long delay times under strong excitation, correspond to coherent Brillouin oscillations and are excluded from subsequent analysis. In Fig. S2(a), the double peak observed in the pseudogap response at excitation fluences above $\mathcal{F}_{\mathrm{P}} \approx 100\mu\mathrm{J/cm}^2$ corresponds to the metallic response, which is characterized by the transient reflectivity with a positive sign (see Fig. 2(e)).

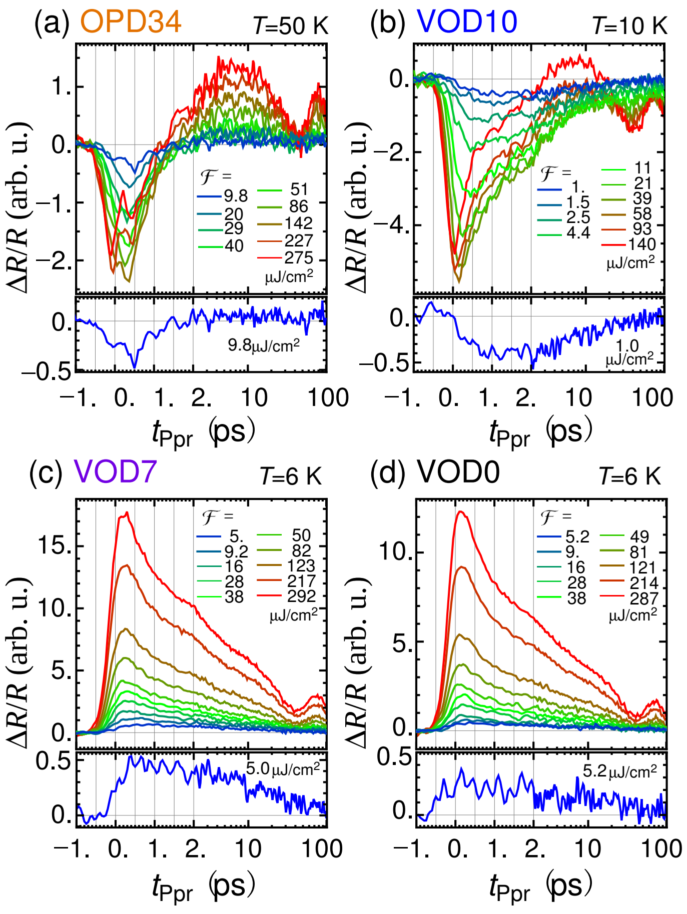


FIG. S2. $\Delta R/R$ at selected $\mathcal{F}_{\mathrm{P}}$ for (a) OPD34 at $T = 50$ K, (b) VOD10 at $T = 10$ K, (c) VOD7 at $T = 6$ K, and (d) VOD0 at $T = 6$ K.

Analogous to the temperature dependence, the data were analyzed using a single-exponential decay approximation. Figure S3 shows the fit parameters for the data shown in Fig. S2, where the amplitudes and the relaxation times are plotted as functions of fluence. In Fig. S3(b), the data at $T = 50$ K are also included for comparison. In OPD34 (Fig. S3(a)) and VOD10 (Fig. S3(b)), the fluence dependence of the amplitude shows saturation characteristics suggesting the pseudogap phase suppression in the photoexcited region – a phenomenon commonly observed in the superconducting and pseudogap carrier dynamics of cuprate superconductors. The fluence dependence of the amplitude is well described by the finite-penetration-depth excitation model [2, 3], which incorporates inhomogeneous pseudogap phase suppression within the photoexcited volume. The solid lines in Fig. S3(a) and (b) represent the fitting results obtained using this model, yielding saturation thresholds of $\mathcal{F}_{\mathrm{th}} = 24.1 \pm 2.3\,\mu\mathrm{J/cm}^2$, $3.3 \pm 0.3\ \mu\mathrm{J/cm}^2$ and $2.9 \pm 0.2\ \mu\mathrm{J/cm}^2$ for OPD34 at $T = 50$ K, VOD10 at $T = 50$ K, and VOD10 at $T = 10$ K, respectively. The linear slope observed at high fluences is attributed to the metallic response that scales linearly with the fluence and has the opposite sign to the PG related response. The observed decrease in $\mathcal{F}_{\mathrm{th}}$ with increasing doping suggests that $\mathcal{F}_{\mathrm{th}}$ scales with the pseudogap energy scale, $\Delta_{\mathrm{PG}}$.

The amplitudes in the VOD7 (Fig. S3(c)) and VOD0 (Fig. S3(d)) samples are dominated by a linear dependence corresponding to the metallic response, with the results of the linear fit to the data indicated by the dashed lines. The fitting is performed using data up to $\mathcal{F}_{\mathrm{P}}$ =300 $\mu\mathrm{J/cm}^2$, as shown in Fig. S2. The result of VOD7 shows a clear deviation from the linear dependence in the low fluence region. The solid lines represent the fitting results obtained using the finite-penetration-depth excitation model[2, 3], in which the saturation thresholds are estimated

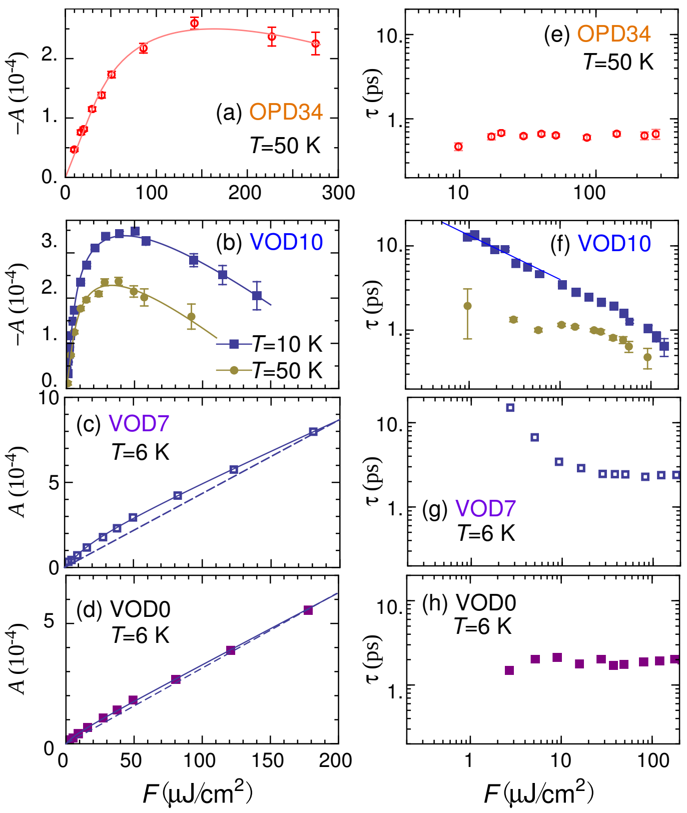


FIG. S3. Amplitude (left) and decay time (right) of the transient reflectivity as functions of fluence for (a, e) OPD34, (b, f) VOD10, (c, g) VOD7, and (d, h) VOD0. Thin solid lines in (a) – (d) indicate fits using the finite-penetration-depth excitation model[2], while the dashed lines in (c) and (d) denote linear fits. The solid line in (f) indicates a power-law fit to the relaxation time, $\tau \propto \mathcal{F}_{\mathrm{P}}^{-z}$.

to be $\mathcal{F}_{\mathrm{th}} = 7.8 \pm 1.3$ $\mu$J/cm$^2$ and $2.4 \pm 1.3$ $\mu$J/cm$^2$ for VOD7 and VOD0, respectively. However, it is essential to consider that these values are influenced by the linear component, which predominantly contributes to the transient reflectivity.

Compared to the amplitude, the fluence dependence of the relaxation time shows qualitatively different behavior when comparing the OPD34 (Fig. S3(e), $T$ =50 K) and VOD10 (Fig. S3 (f), $T$ =10 K) samples. The fluence-independent $\tau$ observed in OPD34 (Fig. S3(e)) is the typical behavior observed for the pseudogap response of various cuprate high-$T_{\mathrm{c}}$ superconductors. In contrast, the relaxation time in VOD10 at $T = 10$ K follows a power-law decrease with increasing fluence as $\tau \propto \mathcal{F}_{\mathrm{P}}^{-z}$. The fitting result for $\tau$ in the fluence range below $\mathcal{F}_{\mathrm{th}}$, where the pseudogap remains partially intact, is shown as a solid line in Fig. S3(f), yielding $z = 0.56$. This fluence dependence of $\tau$, akin to its temperature dependence, indicates a divergence of time scales as $T, \mathcal{F} \to 0$.

A decrease of $\tau$ with increasing fluence is observed also in VOD7 (Fig. S3(g)), but only for the fluence values below the saturation threshold $\mathcal{F}_{\mathrm{th}}$, where the signal is not yet dominated by the metallic response. In contrast, VOD0 exhibits no pronounced slowing of the relaxation dynamics with increasing $\mathcal{F}$, as shown in Fig. S3(h). Combined with the results of the transient response amplitude, these observations indicate that the fluence dependence of VOD0 is primarily dictated by the metallic response that simply scales linearly with $\mathcal{F}$.

## III. RESULTS OF OPD34 IN THE SUPERCONDUCTING REGIME

The characteristics of the superconductivity-related $\Delta R/R$ in the OPD34 sample are summarized in Fig. S4. Figures S4 (a) and (b) show a color density plot of the temperature dependent $\Delta R/R$ and the representative $\Delta R/R$ at selected temperatures, respectively. Compared with the data in Fig. 2(a) ($\mathcal{F}_{\mathrm{P}} = 15$ $\mu$J/cm$^2$), lowering the pump fluence to $\mathcal{F}_{\mathrm{P}} = 2.0$ $\mu$J/cm$^2$ suppresses the negative $\Delta R/R$ associated with the pseudogap response, thereby revealing that the superconducting contribution dominates below $T_{\mathrm{c}}$. Figures S4(c) and S4(d) show the amplitude ($A_{\mathrm{SC}}$) and

relaxation time ($\tau_{SC}$) of the superconducting component, obtained from single-exponential decay fits. The amplitude is well reproduced by an approximation based on the Mattis-Bardeen formula, yielding $T_c = 33 \pm 0.5$K. This estimate is in good agreement with the magnetic susceptibility measurement shown in Fig. S1(a). The residual $A_{SC}$ observed above $T_c$ corresponds to superconducting fluctuations. Figures S4(e) and (f) present the pump-fluence dependence of $A_{SC}$ and $\tau_{SC}$ measured at $T = 10$K. The observed saturation behavior reflects photoinduced superconducting phase destruction and is well captured by a finite-penetration-depth excitation model (solid line), from which a phase destruction threshold fluence of $\mathcal{F}_{th}^{SC} = 0.5 \pm 0.05\mu J/cm^2$ is obtained. This threshold value is nearly an order of magnitude smaller than that for the pseudogap (Fig. S3(a)).

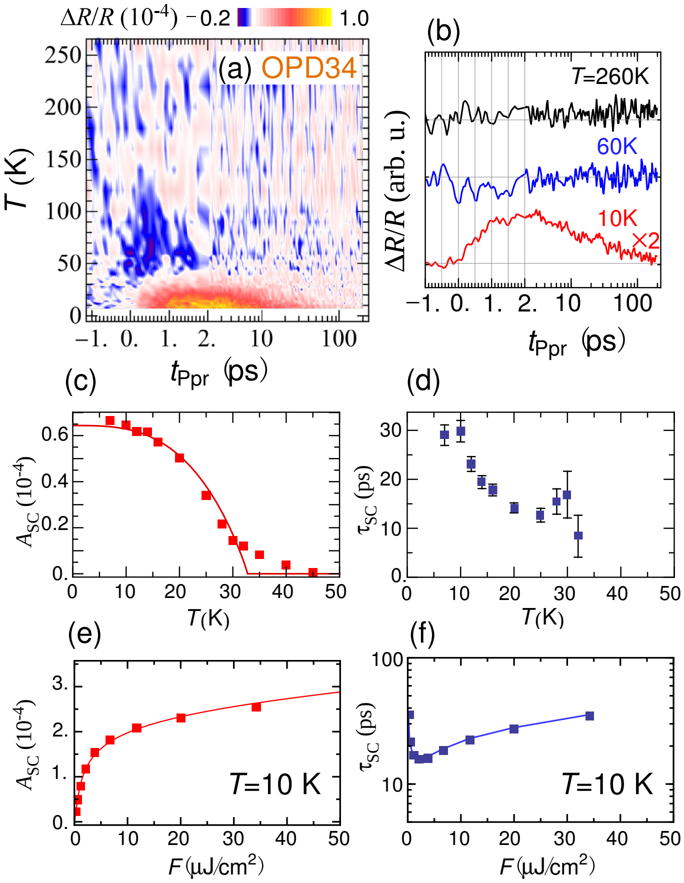


FIG. S4. (a) Color-density plot of the temperature-dependent transient reflectivity $\Delta R/R$ at a pump fluence of $\mathcal{F}_P = 2.0\ \mu J/cm^2$. (b) Representative data of $\Delta R/R$ at selected temperatures. (c, d) Temperature dependence of the amplitude $ASC$ and decay time $\tau_{SC}$ of the superconducting component. The solid line in (c) is a fit using the Mattis-Bardeen formula[4] with a BCS-like gap function, yielding $T_c = 33 \pm 0.5$ K. (e, f) Pump-fluence dependence of $A_{SC}$ and $\tau_{SC}$. The solid line in (e) is a fit to the finite-penetration-depth excitation model[2, 3], giving an estimated destruction threshold of $\mathcal{F}_{th}^{SC} = 0.5 \pm 0.05\ \mu J/cm^2$. The solid line in (f) is a guide to the eye.

Based on $\mathcal{F}_{th}^{SC}$ in the OPD34 sample and assuming that the photoinduced destruction energy of the superconducting phase scales with the square of $T_c$ [5], the saturation thresholds for the superconducting response in the VOD10 and VOD7 samples are estimated to be as low as $0.04\mu J/cm^2$ and $0.02\mu J/cm^2$, respectively. This is consistent with the absence of the SC response in the VOD10 and VOD7 samples, as at these fluences the transient reflectivity amplitude would be on the order of $10^{-7}$, which is comparable to the experimental noise level. Under the realistic excitation conditions, the superconducting response is therefore obscured by the noise and the pseudogap-like response with the larger threshold fluence of $\sim 3\ \mu J/cm^2$.

## IV. ANHARMONIC ENERGY RELAXATION IN THE PHONON-BOTTLENECK MODEL

The pseudogap phonon-bottleneck model [6] is essentially a two-$T$ model where all phonon degrees of freedom with the energy above $2\Delta_{\mathrm{PG}}$ and quasiparticles with the energy $\Delta_{\mathrm{PG}}$ away from the chemical potential are subject to a nonequilibrium temperature $T' = T + \Delta T$. Following the derivation in Kabanov et al. [6] we write the energy-loss rate from the phonons with $\hbar_{\boldsymbol{q}} > 2\Delta_{\mathrm{PG}}$ due to the three-phonon anharmonic processes as,

$$\frac{dE_{>,\mathrm{ph}}}{dt} = \sum_{\boldsymbol{q}(\hbar\omega_{\boldsymbol{q}}>2\Delta_{\mathrm{PG}})} \hbar\omega_{\boldsymbol{q}} I_{\mathrm{ph-ph}}\{\eta_{\omega_{\boldsymbol{q}}}\}, \tag{S1}$$

where $I_{\mathrm{ph-ph}}\{\eta_{\omega_{\boldsymbol{q}}}\}$ is the collision integral (Eq. (16) in Kabanov et al. [6]) with $\eta_\omega$ being the nonequilibrium distribution phonon distribution function. Assuming that the coupling constant is momentum independent we approximate (S1):

$$\begin{aligned}\sum_{\boldsymbol{q}(\hbar\omega_{\boldsymbol{q}}>2\Delta_{\mathrm{PG}})} \hbar\omega_{\boldsymbol{q}} I_{\mathrm{ph-ph}}\{\eta_{\omega_{\boldsymbol{q}}}\} &= 2\pi\hbar w^2 \int_{2\Delta_{\mathrm{PG}}}^{\hbar\omega_{\mathrm{M}}} \omega\rho(\omega)d\omega \\ &\int d\omega_1 \left\{{}^1\!/\!{}_2 \left[(\eta_\omega+1)\,\eta_{\omega_1}\eta_{\omega-\omega_1} - \eta_\omega\,(\eta_{\omega_1}+1)\,(\eta_{\omega-\omega_1}+1)\right]\rho(\omega_1)\rho(\omega-\omega_1)\right. \\ &+ \left.\left[(\eta_\omega+1)\,(\eta_{\omega_1}+1)\,\eta_{\omega+\omega_1} - \eta_\omega\eta_{\omega_1}\,(\eta_{\omega+\omega_1}+1)\right]\rho(\omega_1)\rho(\omega+\omega_1)\right\},\end{aligned} \tag{S2}$$

with the nonequilibrium phonon distribution function,

$$\eta_\omega = \begin{cases} n_\omega(T) & \hbar\omega \le 2\Delta_{\mathrm{PG}} \\ n_\omega(T+\Delta T) & \hbar\omega > 2\Delta_{\mathrm{PG}} \end{cases}. \tag{S3}$$

$\rho(\omega)$ corresponds to the phonon density of states, $n_\omega(T) = \left(e^{-\frac{\hbar\omega}{k_{\mathrm{B}}T}} - 1\right)^{-1}$ to the Bose-Einstein distribution, $w$ to the effective matrix element and $\hbar\omega_{\mathrm{M}}$ to the phonon spectrum cutoff. The excess energy in the high-energy phonons is,

$$\Delta E_{>,\mathrm{ph}} = \int_{2\Delta_{\mathrm{PG}}}^{\hbar\omega_{\mathrm{M}}} \omega\rho(\omega)\left(n_\omega(T+\Delta T) - n_\omega(T)\right)d\omega, \tag{S4}$$

and similar for quasiparticles,

$$\Delta E_{>,\mathrm{qp}} = 2N_0 \int_{\Delta_{\mathrm{PG}}}^{\infty} \epsilon\left(f_\epsilon(T+\Delta T) - f_\epsilon(T)\right)d\epsilon, \tag{S5}$$

where $f_\epsilon(T) = \left(e^{\epsilon/k_{\mathrm{B}}T}+1\right)^{-1}$ is the Fermi function. For simplicity we assume the particle-hole symmetry and an energy independent density of states, $N_0$.

The exponential energy relaxation time, $\tau_E$, is defined as,

$$\frac{dE_{>,\mathrm{ph}}}{dt} = -\frac{\Delta E_{\mathrm{tot}}}{\tau_E} = -\frac{\Delta E_{>,\mathrm{ph}} + \Delta E_{>,\mathrm{qp}}}{\tau_E}. \tag{S6}$$

We define the relaxation time *differently* as in Kabanov et al. [6], assuming that the transient reflectivity is proportional to the density of the photoexcited carriers, $n_{\mathrm{pe}}$, which is proportional to the total deposited laser energy in the weak excitation (linear response) region. In Kabanov et al. [6] the relaxation time was defined through the dynamics of the low-energy phonons temperature, $T$, which does not significantly contribute to the transient reflectivity in the cuprates.

To cover the full $T$ range and take into account a realistic phonon density of states [7] (see Fig. S5) we calculate the integrals (S2) and (S4) numerically. Important parameter of the model is the ratio between the number of phonon and electron degrees of freedom,

$$g_{\mathrm{ph}} = \frac{\int_0^{\omega_c}\rho(\omega)d\omega}{N_0\hbar\omega_{\mathrm{M}}}. \tag{S7}$$

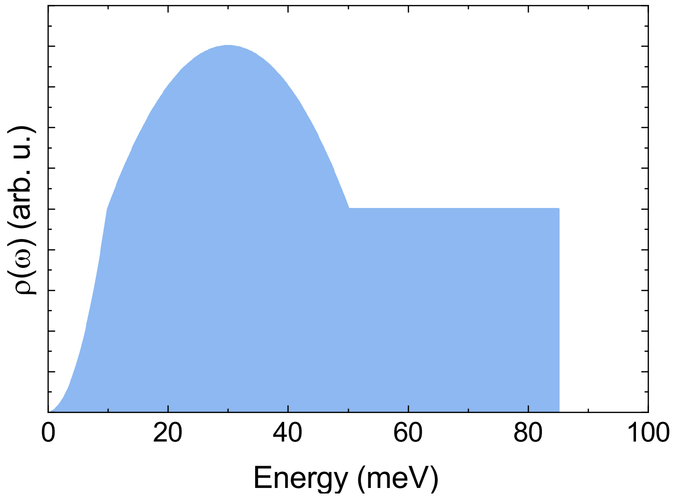


FIG. S5. Approximation of the experimental [7] phonon density of states used for anharmonic phonon energy relaxation rate calculations.

This ratio is estimated to be [6] of the order of $\sim$ 10 in $YBa_2Cu_3O_{7-\delta}$. After checking that the $T$ dependence of $\tau$ does not depend strongly on $g_{\mathrm{ph}}$, we assume, $g_{\mathrm{ph}} = 20$, for the presented calculations. As $\Delta T$ depends exponentially on $\Delta E_{\mathrm{tot}}$ at low $T$ when, $\Delta_{\mathrm{PG}} >> k_{\mathrm{B}}T$, we took care to keep $\Delta E_{\mathrm{tot}}$ small enough to keep $\Delta T/T << 1$ within the relevant $T$ ranges.

[1] M. Berben, S. Smit, C. Duffy, Y.-T. Hsu, L. Bawden, F. Heringa, F. Gerritsen, S. Cassanelli, X. Feng, S. Bron, et al., Phys. Rev. Mater. **6**, 044804 (2022), URL `https://link.aps.org/doi/10.1103/PhysRevMaterials.6.044804`.
[2] P. Kusar, V. V. Kabanov, S. Sugai, J. Demsar, T. Mertelj, and D. Mihailovic, Phys. Rev. Lett. **101**, 227001 (2008), URL `https://link.aps.org/doi/10.1103/PhysRevLett.101.227001`.
[3] M. Naseska, A. Pogrebna, G. Cao, Z. A. Xu, D. Mihailovic, and T. Mertelj, Phys. Rev. B **98**, 035148 (2018), URL `https://link.aps.org/doi/10.1103/PhysRevB.98.035148`.
[4] T. Mertelj, V. V. Kabanov, C. Gadermaier, N. D. Zhigadlo, S. Katrych, J. Karpinski, and D. Mihailovic, Physical Review Letters **102**, 117002 (2009), ISSN 0031-9007, 1079-7114, URL `https://link.aps.org/doi/10.1103/PhysRevLett.102.117002`.
[5] L. Stojchevska, P. Kusar, T. Mertelj, V. V. Kabanov, Y. Toda, X. Yao, and D. Mihailovic, Phys. Rev. B **84**, 180507 (2011), URL `https://link.aps.org/doi/10.1103/PhysRevB.84.180507`.
[6] V. V. Kabanov, J. Demsar, B. Podobnik, and D. Mihailovic, Phys. Rev. B **59**, 1497 (1999), URL `https://link.aps.org/doi/10.1103/PhysRevB.59.1497`.
[7] P. P. Parshin, M. G. Zemlyanov, A. V. Irodova, P. I. Soldatov, and S. K. Sulejmanov, Fizika Tverdogo Tela **38** (1996), URL `https://www.osti.gov/etdeweb/biblio/591229`.
